# Supplementary material for: Stochastic Market Games
Source: arXiv:2207.07388 source file (2022-07-19)
Supplement: Supplementary file 1 [file 7-appendix.tex]

\section{appendix}

% Appendix
\appendix
\section{Supplementary materials}
\begin{algorithm}
  \caption{Balance}\label{alg:markets}
  \begin{algorithmic}[1]
\Procedure{$\texttt{Balance}(\Vec{r}_{t}, B)$}{}
        \For{\texttt{agent ${i}$ in $N$}}
        \For{\texttt{liability ${l}_{i,j}$ in $B_{:,i}$}}
            \If{$\Vec{r}_{i,t} + d^{\texttt{env}} \geq l_{i,j}$}
                \State $\Vec{r}_{i,t} \gets - l_{i,j}$
                \State $\Vec{r}_{j,t} \gets  l_{i,j}$
                \State $B_{i, j} \gets  0$ \Comment{settle debts from $i$ and $j$}
            \EndIf
        \EndFor
    \EndFor
    \State \Return $\Vec{r_t}, B$
\EndProcedure
\end{algorithmic}
\end{algorithm}

\begingroup
\setlength{\tabcolsep}{6.2pt} % Default value: 6pt
 % Default value: 1
\begin{table}[ht]
\centering
\begin{tabular}{l|c}
\hline
\textbf{Parameter}                                  & \textbf{Value} \\ \hline
Environment size                                    & $12 \times 8$  \\
Number agents                                       & 4, 8, 16       \\
Reward high $r_{high}$                              & 5.0            \\
Reward low $r_{low}$                                & 1.0            \\
Number machines                                     & 2              \\
Number machine types                                & 2              \\
Task length                                         & 3              \\
Number steps machine inactive $t_{\text{inactive}}$ & 8              \\ \hline
\end{tabular}
\caption{Key domain parameters: Smartfactory}
\label{tab:key_params}
\end{table}
\endgroup

\begingroup
\setlength{\tabcolsep}{6.2pt} % Default value: 6pt
 % Default value: 1
\begin{table}[ht]
\centering
\begin{tabular}{l|c}
\hline
\textbf{Parameter}                                  & \textbf{Value} \\ \hline
Environment size                                    & $12 \times 8$  \\
Number agents                                       & 4, 8, 16       \\
Reward high $r_{high}$                              & 5.0            \\
Reward low $r_{low}$                                & 1.0            \\
Number initial resources low                        & 5              \\
Number initial resources high                      & 3              \\
\end{tabular}
\caption{Key domain parameters: Refinery}
\label{tab:key_params}
\end{table}
\endgroup

\begingroup
\setlength{\tabcolsep}{6.2pt} % Default value: 6pt
 % Default value: 1
\begin{table}[ht]
\centering
\begin{tabular}{lc}
\hline
\multicolumn{1}{l|}{\textbf{Parameter}}            & \textbf{Value}    \\ \hline
\multicolumn{2}{c}{\textit{Training}}                                           \\ \hline
\multicolumn{1}{l|}{Training episodes}             & 10000 (30000)     \\
\multicolumn{1}{l|}{Steps per episode}             & 200               \\
\multicolumn{1}{l|}{Replay buffer capacity}        & 10000 (30000)     \\
\multicolumn{1}{l|}{Batch size}                    & 32 (64)           \\
\multicolumn{1}{l|}{Steps until target net update} & 500               \\ \hline
\multicolumn{2}{c}{\textit{Exploration}}                                        \\ \hline
\multicolumn{1}{l|}{Function \& $\epsilon$-greedy} & 3                 \\
\multicolumn{1}{l|}{Decay \& linear, per step}     & 8                 \\
\multicolumn{1}{l|}{Start value}                   & 1.0               \\
\multicolumn{1}{l|}{End value}                     & 0.1               \\ \hline
\multicolumn{2}{c}{\textit{Neural Network}}                                     \\ \hline
\multicolumn{1}{l|}{Hidden dense layer}            & 32                \\
\multicolumn{1}{l|}{Hidden dense layer}            & 16                \\
\multicolumn{1}{l|}{Activation function}           & ELU               \\
\multicolumn{1}{l|}{Loss function}                 & Huber (Smooth L1) \\
\multicolumn{1}{l|}{Optimizer}                     & Adam              \\
\multicolumn{1}{l|}{Learning rate}                 & 0.0005            \\ \hline
\end{tabular}
\caption{DQN hyperparameters}
\label{tab:dqn_params}
\end{table}
\endgroup

\begingroup
\setlength{\tabcolsep}{6.2pt} % Default value: 6pt
 % Default value: 1
\begin{table}[ht]
\centering
\begin{tabular}{lc}
\hline
\multicolumn{1}{l|}{\textbf{Parameter}}  & \textbf{Value}                 \\ \hline
\multicolumn{2}{c}{\textit{Training}}                                              \\ \hline
\multicolumn{1}{l|}{Training episodes}   & Training episodes              \\
\multicolumn{1}{l|}{Steps per episode}   & 200                            \\
\multicolumn{1}{l|}{Update time-step}     & 5000                           \\ \hline
\multicolumn{2}{c}{\textit{Neural Network (Actor and Critic)}}                     \\ \hline
\multicolumn{1}{l|}{Hidden dense layer}  & 32                             \\
\multicolumn{1}{l|}{Hidden dense layer}  & 32                             \\
\multicolumn{1}{l|}{Activation function} & Tanh                           \\
\multicolumn{1}{l|}{Loss function}       & Clipped - MSE - 0.01 * entropy \\
\multicolumn{1}{l|}{Epsilon clip}        & 0.2                            \\
\multicolumn{1}{l|}{Training epochs}     & 4                              \\
\multicolumn{1}{l|}{Optimizer}           & Adam                           \\
\multicolumn{1}{l|}{Learning rate}       & 0.002                          \\ \hline
\end{tabular}
\caption{PPO hyperparameters}
\label{tab:ppo_params}
\end{table}
\endgroup
